# Supplementary material for: A Holistic Analysis of Datacenter Operations: Resource Usage, Energy, and Workload Characterization -- Extended Technical Report
Source: arXiv:2107.11832 source file (2021-07-25)
Supplement: Supplementary file 1 [file appendix.tex]

\section{Comparison with previous work on workload characterization}
\label{app:related:workload}

\begin{table*}[th!]
	\caption{Job properties of the analyzed datacenter vs. other environments. Extends the analysis by Amvrosiadis et al.~\cite{DBLP:conf/usenix/AmvrosiadisPGGB18} and demonstrates uniqueness. We mark if a property is present (\checkmark) or absent (\xmark) in the job data.}
	\label{surfing:tbl:properties-comparison-cluster-traces}
	\vcutM
	\adjustbox{max width=\textwidth}{
		\begin{tabular}{|l|m{4cm}|c|c|c|c|c|}
			\hline
			\textbf{Section}                        & \textbf{Characteristic}                                                   & \textbf{Google}   & \textbf{Two Sigma}    & \textbf{Mustang} & \textbf{OpenTrinity}   & \textbf{SURF LISA} \\ \hline \noalign{\smallskip} \hline
			\multirow{2}{*}{Job Characteristics (\cref{surfing:ssct:dataset-outline-job-characteristics})}    & Majority of jobs are small                                                & \checkmark        & \xmark                & \xmark           & \xmark                 & \checkmark             \\ \cline{2-7} 
			& Majority of jobs are short                                                & \checkmark        & \checkmark            & \xmark           & \xmark                 & \checkmark    \\ \hline \noalign{\smallskip} \hline
			\multirow{2}{*}{Workload Heterogeneity (\cref{surfing:ssct:dataset-outline-workload-heterogeneity})} & Diurnal patterns in job submissions                                       & \xmark            & \checkmark            & \checkmark       & \checkmark             & \checkmark             \\ \cline{2-7} 
			& High job submission rate                                                  & \checkmark        & \xmark                & \xmark           & \xmark                 & \checkmark             \\ \hline \noalign{\smallskip} \hline
			\multirow{3}{*}{Resource Utilization (\cref{surfing:ssct:dataset-outline-resource-utilization})}   & Resource over-commitment                                                  & \checkmark        & \checkmark            & \xmark           & \xmark                 & \checkmark             \\ \cline{2-7} 
			& Sub-second job inter-arrival periods                                      & \checkmark        & \checkmark            & \checkmark       & \checkmark             & \checkmark             \\ \cline{2-7} 
			& User request variability                                                  & \xmark            & \checkmark            & \checkmark       & \checkmark             & \xmark    \\ \hline \noalign{\smallskip} \hline
			\multirow{3}{*}{Failure Analysis (\cref{surfing:ssct:dataset-outline-failure-analysis})}       & High fraction of unsuccessful job outcomes                                & \checkmark        & \checkmark            & \xmark           & \checkmark             & \xmark        \\ \cline{2-7} 
			& Jobs with unsuccessful outcomes consume significant fraction of resources & \checkmark        & \checkmark            & \xmark           & \xmark                 & \checkmark    \\ \cline{2-7} 
			& Longer/larger jobs often terminate unsuccessfully                         & \checkmark        & \xmark                & \xmark           & \xmark                 & \checkmark    \\ \hline
		\end{tabular}
	}
	\vcutM
\end{table*}
